# Supplementary material for: Anisotropic hysteretic Hall-effect and magnetic control of chiral domains in the chiral spin states of Pr$_2$Ir$_2$O$_7$
Source: arXiv:1105.2986 source file (2011-05-16)
Supplement: Supplementary file 1 [file Supplementary_Information.pdf]

**Supplementary Information to “Anisotropic hysteretic Hall-effect and magnetic control of chiral domains in the chiral spin states of $Pr_2Ir_2O_7$”**

***The Origin of the hysteresis observed in Hall-effect of $Pr_2Ir_2O_7$ at zero-field***

Figure S1 (a) shows a hysteresis loop of the raw Hall resistance $R=V_H/I$ before the subtraction of the magnetoresistance component. Figure S1(b) shows the Hall resistance $R_{xy}$ obtained by subtracting the magnetoresistance contribution, for both increasing (blue trace) and decreasing (clear blue trace) field sweeps.

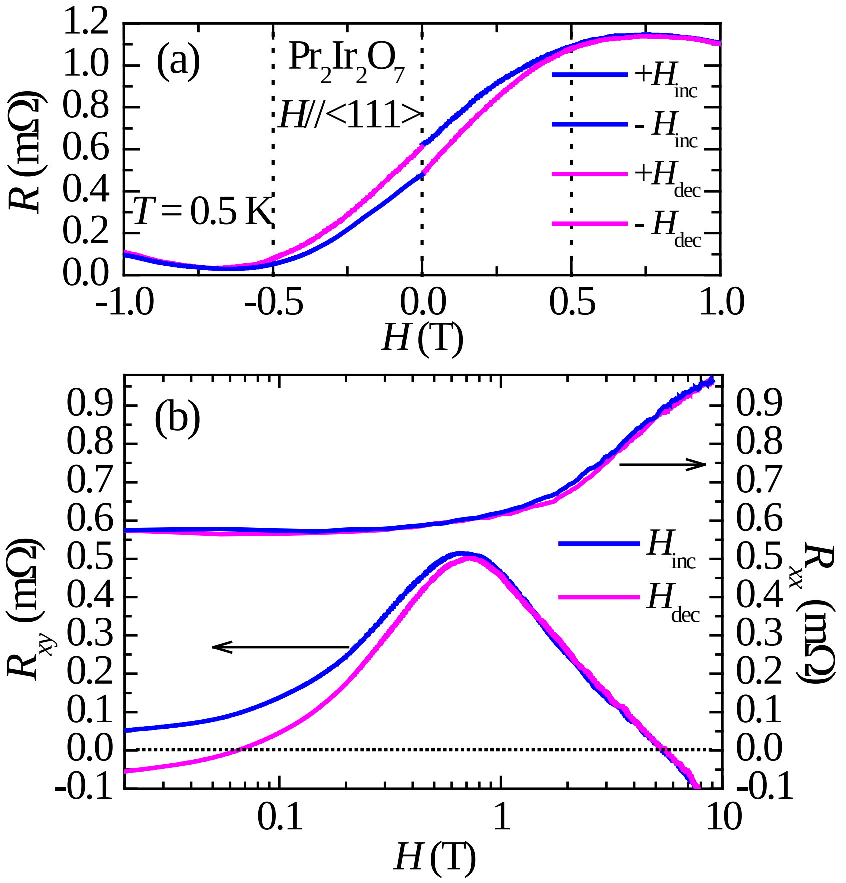


< FIG. S1> (a) Raw Hall signal $R = V_H / I$, where $V_H$ is the Hall signal and $I$ is the injected current, for a $Pr_2Ir_2O_7$ single crystal as a function of magnetic field $H$ and at a temperature $T$ = 0.5 K, respectively for increasing (blue) and decreasing (magenta)

field scans along both field directions. H was applied along the [111] direction. (b) The magnetoresistive $R_{xx}$ = ($V_H$ (+$H$)+ $V_H$ (−$H$))/2$I$ and the Hall resistivity $R_{xx}$ =($V_H$ (+$H$) − $V_H$ (−$H$))/2$I$ components superimposed onto R as a function of magnetic field $H$, and respectively for increasing and decreasing field sweeps. Notice the marked hysteresis in $R_{xy}$, particularly when compared to $R_{xx}$.

Notice the marked hysteresis seen around zero field, although $T$ = 0.5 K is considerably larger than the reported spin freezing temperature $T_f$ = 0.12-0.3 K for this compound [S1,S2]. The residual value of Hall resistance at zero field for both increasing and decreasing field sweep traces have the same magnitude but opposite sign with respect to each other. In the conventional definition of the Hall constant $R_H = R_{xy} \cdot t/H$, where $t$ is the sample thickness, this behaviour would lead to a divergent Hall constant at zero field. For the sake of comparison, we show in Fig S1 (b) the magnetoresistance component $R_{xx}$ superimposed onto the original raw Hall signal as a function of magnetic field. Notice how the hysteresis observed in $R_{xy}$ is far more pronounced. Magnetic susceptibility and magnetization measurements shown in Ref. [S1], indicate that neither conventional magnetic order, such as ferromagnetism, nor glassy behaviour is responsible for the behaviour shown here at $T$ = 0.5 K > $T_f$.

[S1] Nakatsuji, S. *et al.* Metallic Spin-Liquid Behavior of the Geometrically Frustrated Kondo Lattice $Pr_2Ir_2O_7$. *Phys. Rev. Lett.* **96**, 087204 (2006).

[S2] Machida, Y., *et al.* Unconventional Anomalous Hall Effect Enhanced by a Noncoplanar Spin Texture in the Frustrated Kondo Lattice $Pr_2Ir_2O_7$. *Phys. Rev. Lett.* **98**, 057203 (2007).
